# Supplementary material for: A Christoffel function weighted least squares algorithm for collocation approximations
Source: arXiv:1412.4305 source file (2016-01-29)
Supplement: Supplementary file 1 [file appendix.tex]

\section{Matrix inequalities}
We attempt to generalize the results from [Tropp, FCM] regarding matrix inequalities. Let $\mathbf{X}_k \in \R^{d \times d}$ be a sequence of independent positive semi-definite matrices. Assume
\begin{align}\label{eq:X-spectrum-assumptions}
  P\left[ \lambda_{\textrm{max}}(\mathbf{X}_k) \leq 1 \right] &= p, &
  P\left[ 1 < \lambda_{\textrm{max}}(\mathbf{X}_k) \leq R \right] &= 1-p.
\end{align}
Consider the maximum spectrum of the expected sum:
\begin{align*}
  \mu_{\textrm{max}} \triangleq \lambda_{\textrm{max}}\left( \sum_k \E \mathbf{X}_k \right)
\end{align*}
We want ultimately to gain an understanding of the bounds
\begin{align*}
  P \left[ \lambda_{\textrm{max}} \left( \sum_{k} \mathbf{X}_k \right) \geq (1 + \delta) \mu_{\textrm{max}}\right]
\end{align*}

To begin, we can easily generalize the Chernoff mgf bound (Lemma 5.8 of [Tropp]). The original bound says: assume $\lambda_{\textrm{max}}(\mathbf{X}) \leq 1$. Then for all $\theta \in \R$:
\begin{align}\label{eq:tropp-chernoff-mgf}
  \E e^{\theta \mathbf{X}} \preccurlyeq \mathbf{I} + (e^{\theta} - 1) \E \mathbf{X}
\end{align}
We can use the tower rule to obtain a more refined estimate: assume \eqref{eq:X-spectrum-assumptions}, and let the event $A$ be defined as $A = \left\{\lambda_{\textrm{max}}(\mathbf{X}_k) \leq 1\right\}$. Then:
\begin{align*}
  \E e^{\theta \mathbf{X}} &= \E \left[ e^{\theta \mathbf{X}}\, |\, A\right] P\left[ A \right] + \E \left[ e^{\theta \mathbf{X}}\, |\, A^c \right] P\left[ A^c \right] \\ 
                           &\preccurlyeq \left[ \mathbf{I} + (e^\theta - 1) \E\mathbf{X} \right] p + \left[ \mathbf{I} + (e^{R \theta} - 1) \frac{1}{R} \E \mathbf{X} \right] (1-p) \\
                           &= \mathbf{I} + \left( p (e^\theta - 1) + \frac{1-p}{R} (e^{R \theta} - 1)\right) \E \mathbf{X}\\
  &\triangleq \mathbf{I} + g(\theta) \E \mathbf{X}
\end{align*}
The first equality uses basic properties of conditional expectation, and the second uses $P[A]$ defined by \eqref{eq:X-spectrum-assumptions} along with the vanilla Chernoff mgf bound \eqref{eq:tropp-chernoff-mgf} with appropriate $R$-scaling.

Proceeding as in [Tropp], we begin with (5.1) which in turn uses Corollary 3.9:
\begin{align*}
P \left[ \lambda_{\textrm{max}} \left( \sum_{k} \mathbf{X}_k \right) \geq t\right] \leq d \,\exp \left( -\theta t + n \,\log \left( 1 + \frac{1}{n} g(\theta) \mu_{\textrm{max}}\right)\right),
\end{align*}
which is true for all $\theta > 0$. Using the fact that $\log (1 + x) \leq x$ for $x > -1$, we have
\begin{align*}
P \left[ \lambda_{\textrm{max}} \left( \sum_{k} \mathbf{X}_k \right) \geq t\right] \leq d \,\exp \left( -\theta t + g(\theta) \mu_{\textrm{max}}\right)
\end{align*}
Now we set $t \gets (1+\delta) \mu_{\max}$, whicy yields
\begin{align*}
  P \left[ \lambda_{\textrm{max}} \left( \sum_{k} \mathbf{X}_k \right) \geq t\right] \leq d \,\exp \left( -\theta (1+\delta) \mu_{\max} + g(\theta) \mu_{\textrm{max}}\right)
\end{align*}
The value of $\theta$ that minimizes this expression solves the equation
\begin{align*}
  g'(\theta) = 1 + \delta, \hskip 10pt \Longrightarrow \hskip 10pt p e^\theta + (1-p) e^{R\theta} = 1 + \delta
\end{align*}
We know that if $p=1$, then $\theta = \log(1 + \delta)$ and if $p = 0$ then $\theta = \frac{1}{R} \log(1 + \delta)$. But I don't know how to solve this for general $p$....

Note that we can trivially extend the [Tropp] results:
\begin{align*}
  P \left[ \lambda_{\textrm{max}} \left( \sum_{k} \mathbf{X}_k \right) \geq t\right] &= 
  P \left[ \lambda_{\textrm{max}} \left( \sum_{k} \mathbf{X}_k \right) \geq t\,|\, A \right] P[A] + P \left[ \lambda_{\textrm{max}} \left( \sum_{k} \mathbf{X}_k \right) \geq t\,|\, A^c \right] P[A^c] \\
  &\leq d p \left[ \frac{e^{\delta}}{(1+\delta)^{1+\delta}}\right]^{\mu_{\max}} + 
        d (1-p) \left[ \frac{e^{\delta}}{(1+\delta)^{1+\delta}}\right]^{\mu_{\max}/R}
\end{align*}
